# Supplementary material for: Capabilities for Better ML Engineering
Source: arXiv:2211.06409 source file (2023-02-10)
Supplement: Supplementary file 1 [file 6-appendices.tex]

\section{Experiment Setting}
\label{appendix:experiment}

% We have discussed capabilities' broad applications for ML engineering across different stages, stakeholders, and attributes.
% However, there still exist many challenges in integrating capabilities into ML engineering. 
% We next list challenges and discuss their research opportunities.

\paragraph{Data}
We use the \textsc{Amazon-wilds} dataset~\cite{pmlr-v139-WILDS} for sentiment analysis.
The dataset consists of Amazon reviews of many different categories and their ratings.
We select the \textsc{Home-and-kitchen} category for training and ten other categories for evaluation. 
In domain adaptation, the \textsc{Home-and-kitchen} category would be referred to as source domain, while the other categories are target domains. 
Following previous work in domain adaptation~\cite{blitzer-etal-2007-biographies}, we convert ratings to binary labels (positive when >3, negative when <3) and sample a balanced dataset for each category (domain).

\paragraph{Model}
% We select two model architectures for our evaluation: LSTM and BERT~\cite{bhargava2021generalization, DBLP:journals/corr/abs-1908-08962}.
% We trained 200 LSTM models and 
To obtain a series of models with different accuracy, we fine-tuned a pre-trained BERT model~\cite{bhargava2021generalization, DBLP:journals/corr/abs-1908-08962} 100 times on different random seeds.

\paragraph{Method}
Our goal is to observe the correlations between model accuracy across source domain and target domains,
as well as how extra information (e.g., accuracy on capability test suites) would affect the correlations.

We first use a linear model to compute the correlations of accuracy between source domain and target domains, without any extra variables.
We then introduce three sets of variables to the linear model:

\begin{enumerate}
    \item \textit{Capability test suite accuracy}: we first selected eight capabilities for sentiment analysis based on an existing study~\cite{barnes-etal-2019-sentiment}. We instantiated these capabilities by slicing the source domain dataset on their corresponding keywords (see Tab.~\ref{tab:cap-inst}).
    We computed the models' accuracy on the capability test suites and removed five of them due to collinearity. 
    The final capabilities we used are \textit{shifter}, \textit{modality}, and \textit{comparative}.
    \item \textit{Random subset accuracy}: we selected three random subsets from the source dataset. These subsets are of the same size as the three capability test suites. We computed the models' accuracy on the random subsets.
    \item \textit{Noisy accuracy}:  we added random Gaussian noise to the models' validation accuracy.
    % \item \textit{Long text subset's accuracy}: we selected texts longer than 150 tokens from source dataset and computed models' accuracy on the slice.
\end{enumerate}

For the last two settings, we repeated the process on 100 different random seeds and averaged their results.

We then fit the linear model with these extra variables for each setting.
We looked at adjusted $R^2$ to see whether the model has a better fit (i.e., whether these extra variables help predict out-of-distribution accuracy). 
\footnote{$R^2$ represents the proportion of the variance that could be explained by input variables. 
Higher $R^2$ implies a better fit of the linear model and higher predictive power of input variables.
We used adjusted $R^2$ to compensate for the effect of extra degrees of freedom. It only increases if the new variable enhances the model above what would be obtained by chance.}
We also performed \textsc{ANOVA} testing to see whether the improvement is statistically significant. 

To understand the relation between capability predictiveness and distribution distance, we followed the method from previous work~\cite{blitzer-etal-2007-biographies} to compute a proxy $\mathcal{A}$-distance between different domains.

% \section{Experiment Results}
% We found that capabilities better help predict model generalization compared to all other baselines.
% The linear model's adjusted $R^2$ increases (statistically significantly) in 50\% domains with extra variables from capabilities.
% In contrast, the best baseline (random subsets) only increases adjusted $R^2$ in 20\% domains on average (see Fig.~\ref{fig:improvement} for details).

% For finetuned BERT models, that adjustd $R^2$ increases significantly in 5 out of 10 casese

% We found that different capabilities add different information for prediction.
% Some capabilities (e.g., \textit{negation}) produce too many test cases, which leads to an uninformative distribution close to the original dataset.
% Different capabilities could also augment each other: 
% \textit{shifter} improves predictive power in 2 cases, but adding \textit{modality} further increases predictive power in 4 cases.

% We found that capabilities' predictiveness correlates with distribution distance (see Fig.~\ref{fig:distance}). 
% The further the domain is, the better capabilities could help predict generalization.
% We hypothesize that this might be due to the fact that if a target domain is too close to the source domain,
% there is little room left for improvement.
